# Supplementary material for: Dataset Distillation for Handwritten Text Recognition: An Empirical Study
Source: arXiv:2611.21054 source file (2026-11-17)
Supplement: Supplementary file 1 [file supp_objective.tex]

IAM & 62 & 0.980 [0.979, 0.982] & 0.983 [0.982, 0.984] & 1.000 [1.000, 1.000] & 0.995 [0.994, 0.996] & 1.000 [1.000, 1.000] & 1.002 [1.001, 1.002] \\
IAM & 308 & 0.997 [0.996, 0.997] & 0.997 [0.997, 0.997] & 1.000 [1.000, 1.000] & 0.999 [0.999, 0.999] & 1.000 [1.000, 1.000] & 1.000 [1.000, 1.000] \\
IAM & 616 & 0.998 [0.998, 0.999] & 0.999 [0.999, 0.999] & 1.000 [1.000, 1.000] & 0.999 [0.999, 0.999] & 1.000 [1.000, 1.000] & 1.000 [1.000, 1.000] \\
GW & 4 & 0.704 [0.688, 0.721] & 0.770 [0.762, 0.778] & 0.992 [0.991, 0.993] & 0.969 [0.965, 0.974] & 1.001 [1.001, 1.002] & 0.982 [0.977, 0.986] \\
GW & 18 & 0.917 [0.911, 0.924] & 0.924 [0.922, 0.925] & 0.998 [0.998, 0.999] & 0.994 [0.992, 0.995] & 0.999 [0.999, 0.999] & 0.998 [0.998, 0.999] \\
GW & 36 & 0.948 [0.945, 0.952] & 0.959 [0.958, 0.961] & 0.999 [0.999, 0.999] & 0.993 [0.991, 0.995] & 1.000 [0.999, 1.000] & 1.000 [1.000, 1.000] \\
READ\,2016 & 84 & 0.977 [0.976, 0.979] & 0.975 [0.973, 0.976] & 1.000 [0.999, 1.000] & 0.996 [0.996, 0.997] & 1.000 [1.000, 1.000] & 0.998 [0.998, 0.999] \\
READ\,2016 & 418 & 0.995 [0.994, 0.995] & 0.996 [0.995, 0.996] & 1.000 [1.000, 1.000] & 0.999 [0.999, 0.999] & 1.000 [1.000, 1.000] & 1.000 [1.000, 1.000] \\
READ\,2016 & 835 & 0.997 [0.997, 0.997] & 0.998 [0.998, 0.998] & 1.000 [1.000, 1.000] & 1.000 [0.999, 1.000] & 1.000 [1.000, 1.000] & 1.000 [1.000, 1.000] \\
LAM & 198 & 0.992 [0.991, 0.992] & 0.992 [0.991, 0.993] & 1.000 [1.000, 1.000] & 0.999 [0.998, 0.999] & 1.000 [1.000, 1.000] & 1.000 [1.000, 1.000] \\
LAM & 991 & 0.998 [0.998, 0.998] & 0.998 [0.998, 0.998] & 1.000 [1.000, 1.000] & 1.000 [1.000, 1.000] & 1.000 [1.000, 1.000] & 1.000 [1.000, 1.000] \\
LAM & 1983 & 0.999 [0.999, 0.999] & 0.999 [0.999, 0.999] & 1.000 [1.000, 1.000] & 1.000 [1.000, 1.000] & 1.000 [1.000, 1.000] & 1.000 [1.000, 1.000] \\
